# Supplementary material for: Bayesian hierarchical modelling for inferring genetic interactions in yeast
Source: arXiv:1508.03454 source file (2015-08-14)
Supplement: Supplementary file 1 [file appendix.tex]

\appendix
\section{Priors for SHM, IHM and JHM in Section~\ref{Application_data}}
\FloatBarrier
\restylefloat{table}
\setcounter{figure}{0}
\setcounter{table}{0}
\begin{table}[H]
\caption{Hyperparameter values for the SHM, IHM and JHM. \label{table:priors}}
\centering 
\resizebox{!}{0.9in}{%
\npdecimalsign{.}
\nprounddigits{2}
\centering 
\begin{tabular}{c n{2}{2} c n{2}{2} c n{2}{2} c n{2}{2}}
    \hline
\noalign{\vskip 0.4mm} 
		\multicolumn{2}{c}{SHM \& JHM} &\multicolumn{2}{c}{SHM \& JHM}& \multicolumn{2}{c}{JHM} & \multicolumn{2}{c}{IHM}\\
Parameter Name  & \multicolumn{1}{c}{Value} & Parameter Name  & \multicolumn{1}{c}{Value} & Parameter Name  & \multicolumn{1}{c}{Value}& Parameter Name  & \multicolumn{1}{c}{Value}\\ \hline
$\tau^{K,\mu}$ & 2.20064039227566   & $\eta^{r,p}$ & 0.133208648543871 &$\alpha^{\mu}$ & 0 & $Z_{\mu}$ & 3.65544229414228  \\ 
$\eta^{\tau,K,p}$ & 0.0239817523340161  &       $\nu^{\mu}$ & 19.8220570630669 &  $\eta^{\alpha}$ & 0.25 & $\eta^{Z,p}$ & 0.697331530063874 \\  
 $\eta^{K,o}$ & -0.79421175992029 & $\eta^{\nu,p}$ & 0.0174869367984725 &$\beta^{\mu}$ & 0 &  $\eta^{Z}$ & 0.104929506383255 \\ 
  $\psi^{K,o}$ & 0.610871036009521 &  $P^{\mu}$ & -9.03928728018792 &  $\eta^{\beta}$ & 0.25  &   $\psi^{Z}$ & 0.417096744759774 \\  
     $\tau^{r,\mu}$ &  3.64993037268256 &  $\eta^{P}$ & 0.469209463148874 &  $p$ & 0.05 & $\eta^{\nu}$ & 0.101545024587153 \\   
 $\eta^{\tau,r,p}$ &  0.0188443648965434 &&&$\eta^{\gamma}$ & -0.79421175992029 &  $\psi^{\nu}$ & 2.45077729037385 \\ 
$\eta^{r,o}$ & 0.468382435659566  &&& $\psi^{\gamma}$ & 0.610871036009521 &    $\nu^{\mu}$ & 2.60267545154548 \\ 
 $\psi^{r,o}$ & 0.0985295312016232  &&&  $\eta^{\omega}$ & 0.468382435659566 &    $\eta^{\nu,p}$ &0.0503202367841729  \\ 
  $\eta^{\nu}$ & -0.834166609695065  &&& $\psi^{\omega}$ & 0.0985295312016232 &    $\alpha^{\mu}$ & 0 \\ 
 $\psi^{\nu}$ & 0.855886535578262  &&& $\eta^{\tau,K}$ &  2.20064039227566&    $\eta^{\alpha}$ & 0.309096075088720 \\   
  $K^{\mu}$ & -2.01259579112252  &&&   $\psi^{\tau,K}$ & 0.0239817523340161 &    $p$ & 0.05 \\ 
 $\eta^{K,p}$ & 0.032182397822033  &&& $\eta^{\tau,r}$ & 3.64993037268256 & $\eta^{\gamma}$ & 0.104929506383255 \\ 
    $r^{\mu}$ & 0.97398228941848  &&&   $\psi^{\tau,r}$ & 0.0188443648965434 &  $\psi^{\gamma}$ & 0.417096744759774 \\  
    \hline
    \end{tabular}
    \npnoround
		}
\end{table}
